# Supplementary material for: Grounding Stylistic Domain Generalization with Quantitative Domain Shift Measures and Synthetic Scene Images
Source: arXiv:2405.15961 source file (2024-05-24)
Supplement: Supplementary file 1 [file 10_appendix.tex]

\newpage
\appendix

% \begin{figure*}[t]
% \centering
% \includegraphics[width=\linewidth]{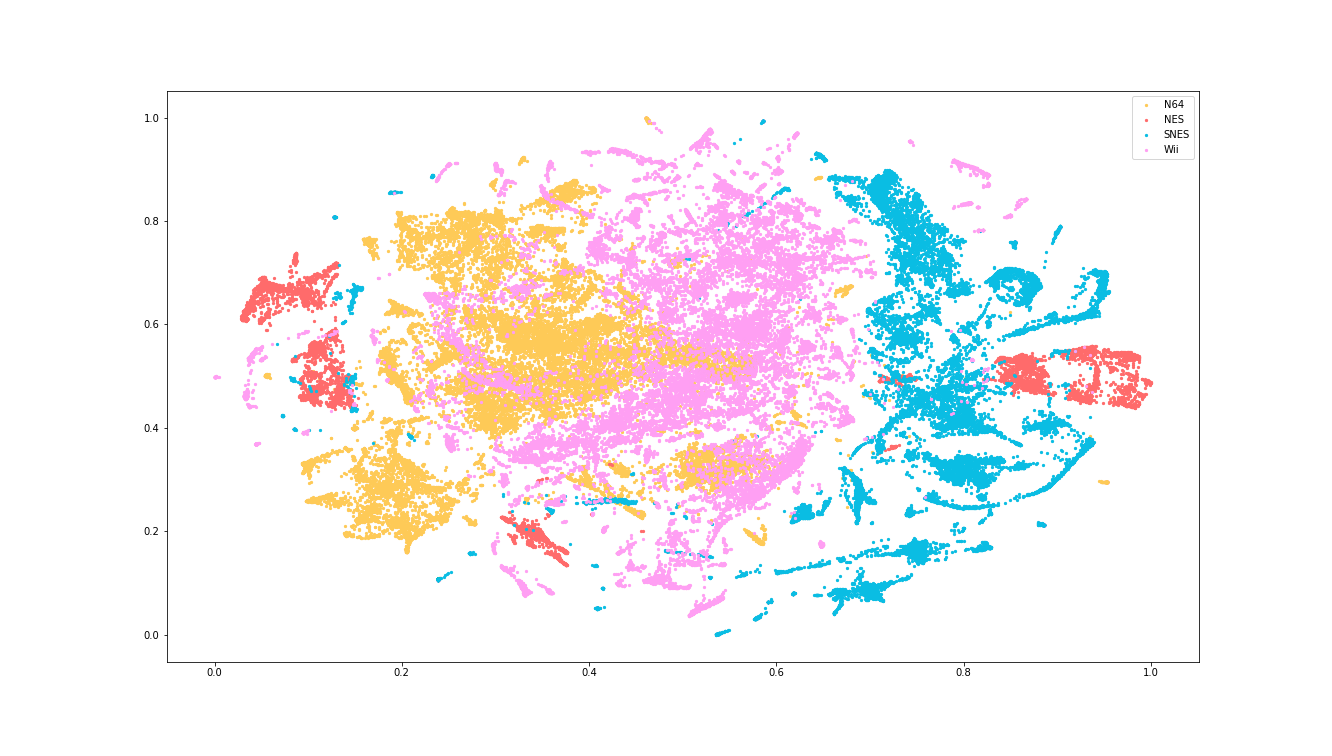} 
% \caption{t-SNE plot of SuperMarioDomains' features extracted by ResNet50 with ImageNet1K pre-training.}
% \end{figure*}

\section{Reproducibility}
\label{app: settings}

\textbf{Data augmentation. }We use the same data augmentation settings consistent with ERM\cite{gulrajani2021in} and MIRO\cite{miro}. For training data, each image is cropped of random size and aspect ratio, resized to 224×224 pixels, applied random horizontal flips, applied random color jitter, applied grayscaling the image with 10\% probability, and normalized using the ImageNet channel means and standard deviations. For test data, only resizing to 224x224 and the ImageNet-based normalization are applied.

\textbf{Hyperparameter tunning.} We use a universal batch size of 16, and the Adam optimizer\cite{kingma2014adam} for all experiments. Crucial hyperparameters including learning rate, dropout, and weight decay are consistent with the ones reported in MIRO. Each benchmark uses a different combination of hyperparameters as following. Experiments on PACS and OfficeHome use 2 NVIDIA V100 GPUs, while experiments on DomainNet use 2 NVIDIA A100 GPUs. 

For all the baseline methods including the original MIRO and our 2-phase MIRO2, we copy the hyperparameters used in the original MIRO per benchmark:
\begin{table}[h]
\centering
\begin{tabular}{ l|rrr } 
 \toprule
 \textbf{Benchmark} & \textbf{PACS} & \textbf{OfficeHome} & \textbf{DomainNet} \\ 
 \midrule
 Learning rate & $3 \times 10^{-5}$ &  $3 \times 10^{-5}$ &  $3 \times 10^{-5}$ \\ 

 Dropout& 0.0 & 0.1 & 0.1 \\ 

 Weight decay& 0.0 & $1 \times 10^{-6}$ & 0.0 \\ 

 $\lambda$ & 0.01 & 0.1 & 0.1 \\ 
 \bottomrule
\end{tabular}
\caption{Hyperparameters for SuperMarioDomains baseline and oracle pre-training with MIRO2.}
\label{table: hp1}
\end{table}

When we perform with the additional last-layer KL-Divergence regularization term $\lambda_{\mathrm{KL}}$, such as MIRO2+KL for oracle pre-training experiments and MIRO+KL in ablation studies, we use a slightly altered set of hyperparameters:

\begin{table}[h]
\centering
\begin{tabular}{ l|rrr } 
 \toprule
 \textbf{Benchmark} & \textbf{PACS} & \textbf{OfficeHome} & \textbf{DomainNet} \\ 
 \midrule
 Learning rate & $3 \times 10^{-5}$ &  $3 \times 10^{-5}$ &  $3 \times 10^{-5}$ \\ 

 Dropout& 0.0 & 0.0 & 0.0 \\ 

 Weight decay& 0.0 & 0.0 & 0.0 \\ 

 $\lambda$ & 0.001 & 0.1 & 0.01 \\ 
 $\lambda_{\mathrm{KL}}$ & 0.001 & 0.1 & 0.05 \\ 
 \bottomrule
\end{tabular}
\caption{Hyperparameters for oracle pre-training with MIRO2+KL and ablation studies with MIRO+KL.}
\label{table: hp2}
\end{table}

\begin{table*}[t]\centering
\resizebox{1.0\linewidth}{!}{
\begin{tabular}{l|ll|l|rrrrrrrr}\toprule
\multirow{2}{*}{\textbf{Algorithm}}&\multicolumn{2}{c|}{Oracle}&\multicolumn{1}{c|}{Featurizer}&\multicolumn{6}{c}{DomainNet Target Domains}  &&\\
&\multicolumn{1}{c}{Method} &\multicolumn{1}{c|}{ Pt. Data} & \multicolumn{1}{c|}{ Pt. Data} &Painting & Infograph &  Clipart& Quickdraw &  Real  &  Sketch &   Avg.  &$\Delta_{D}$  \\\midrule
% \multicolumn{15}{l}{\textit{All backbone featurizers are initialized from scratch, including the target task featurizer in Phase 2.} }\\\midrule

%    & 00.0\errmath{0.0} & 00.0\errmath{0.0}& 00.0\errmath{0.0}& 00.0\errmath{0.0}& 00.0\errmath{0.0}& 00.0\errmath{0.0}& 00.0\errmath{0.0} &+0.0 \\ 
ERM &- &-    &ImageNet1K                        & 59.1\errmath{0.0} & 19.1\errmath{0.2}& 46.2\errmath{0.1}& 13.1\errmath{0.0}& 60.9\errmath{0.0}& 50.5\errmath{0.0}& 41.5\errmath{0.1} &- \\ 
SagNet &- &- &ImageNet1K                        & 58.5\errmath{0.0} & 18.5\errmath{0.3}& 48.2\errmath{0.0}& 13.0\errmath{0.0}& 58.7\errmath{0.2}& 47.1\errmath{0.0}& 40.6\errmath{0.1} &- \\ 
RandConv &- &- &ImageNet1K                      & 57.5\errmath{0.0} & 17.6\errmath{0.4}& 46.0\errmath{0.1}& 12.9\errmath{0.0}& 58.8\errmath{0.1}& 46.8\errmath{0.0}& 39.9\errmath{0.1} &- \\ 
MIRO &- &ImageNet1K &ImageNet1K                 &59.6\errmath{0.2} &21.8\errmath{0.1} &51.3\errmath{0.1} &15.2\errmath{0.3} &63.7\errmath{0.0} & 45.0\errmath{0.1} &42.8\errmath{0.1} &+0.0\\
\midrule   

MIRO2           &ERM  &SMD(Ours)  &ImageNet1K   & 62.2\errmath{0.0} & 21.1\errmath{0.0}& \textbf{51.4}\errmath{0.0}& 13.9\errmath{0.1}& 63.9\errmath{0.0}& \textbf{53.3}\errmath{0.0}& 44.3\errmath{0.0} &+1.5 \\ 
(Ours)          &MIRO &SMD(Ours)  &ImageNet1K   & 62.0\errmath{0.3} & 21.2\errmath{0.2}& 51.2\errmath{0.1}& 14.4\errmath{0.1}& 63.9\errmath{0.0}& \textbf{53.3}\errmath{0.0}& 44.3\errmath{0.1} &+1.5 \\ \midrule
MIRO2+KL        &ERM  &SMD(Ours)   &ImageNet1K  & \textbf{62.3}\errmath{0.1} & \textbf{21.3}\errmath{0.0}& 51.3\errmath{0.0}& \textbf{14.7}\errmath{0.0}& \textbf{64.0}\errmath{0.1}& 53.1\errmath{0.1}& \textbf{44.5}\errmath{0.0} &\textbf{+1.7} \\ 
(Ours)          &MIRO &SMD(Ours)   &ImageNet1K  & 62.0\errmath{0.3} & 21.2\errmath{0.3}& 51.0\errmath{0.1}& \textbf{14.7}\errmath{0.3}& \textbf{64.0}\errmath{0.1}& \textbf{53.3}\errmath{0.0}& 44.3\errmath{0.1} &+1.5 \\ 

\bottomrule

\end{tabular}
}
\newline
\caption{Out-of-domain DG performances on DomainNet. Consistent with the latter half of Table \ref{tab: miro2-results}, the \textbf{best results} are highlighted in bold. $\Delta_{D}$ stands for the average accuracy improvement over the SOTA results on DomainNet. All average accuracies and errors are reported from three best trials. }\label{tab: domainnet-results}
\end{table*}

\section{Performance on the DomainNet Benchmark of Oracle Pre-training}
In addition to PACS and OfficeHome, we evaluate the DG performance of our methods on the more challenging DomainNet benchmark \citep{domainnet} using the same leave-one-out cross-validation. DomainNet consists of 587K images in 6 image style domains and 345 object classes. We hence choose the whole data from 5 domains as sources and the remaining 1 domain for testing at a time. We similarly randomly split 20\% out of each source domain for in-domain validation. We report the performances by the MIRO2/MIRO2+KL methods with SMD oracle pre-training in comparison with the baseline methods. We assume the featurizers used in the baseline methods as well as in Phase 2 of MIRO2/MIRO2+KL are ResNet50 backbones initialized with ImageNet1K pre-trained weights. Experiment configurations on DomainNet are included in Table \ref{table: hp1} and \ref{table: hp2}.

The results on the DomainNet benchmark in Table \ref{tab: domainnet-results} resonates with our conclusions in Sec \ref{section-miro2}. Methods with the additional oracle pre-training phase such as MIRO2 and MIRO2+KL enjoy a comfortable lead on DomainNet, with an improvement of at least +1.5 over the baseline MIRO method on the Average category. Moreover, better overall results on DomainNet can be achieved by using the additional KL regularization term alongside oracle pre-training, claiming the top Average performance at 44.5, at +1.7 over the MIRO baseline.

\section{Ablation Studies}
For all the following ablation studies, we assume the featurizer used in Phase 2 of MIRO2/MIRO2+KL is initialized with ImageNet1K pre-trained weights.

\subsection{The Effects of the KL Regularization Term}
We study the singled-out impact by applying the last-layer KL regularization loss $\lambda_{\mathrm{KL} }\Lagr_{\mathrm{KL}}$ to the original baseline MIRO where both its oracle and featurizer use ImageNet1K pre-training. We compare the performances on the three chosen benchmarks, PACS, OfficeHome, and DomainNet. 

\begin{table*}[t]\centering

\begin{tabular}{l|ll|l|rrrr}\toprule
\multirow{2}{*}{\textbf{Algorithm}}&\multicolumn{2}{c|}{Oracle}&\multicolumn{1}{c|}{Featurizer}&\multicolumn{4}{c}{Benchmark Avg. }  \\
&\multicolumn{1}{c}{Method} &\multicolumn{1}{c|}{ Pt. Data} &  \multicolumn{1}{c|}{ Pt. Data} &PACS & OfficeHome & DomainNet & Avg.\\\midrule
% \multicolumn{15}{l}{\textit{All backbone featurizers are initialized from scratch, including the target task featurizer in Phase 2.} }\\\midrule

%    & 00.0\errmath{0.0} & 00.0\errmath{0.0}& 00.0\errmath{0.0}& 00.0\errmath{0.0}& 00.0\errmath{0.0}} &+0.0 \\ 
MIRO  &-&ImageNet1K &ImageNet1K&87.7\errmath{0.1} &68.9\errmath{0.1} &42.8\errmath{0.1} &66.5\\
MIRO+KL &- &ImageNet1K &ImageNet1K &87.2\errmath{0.1} &69.7\errmath{0.3} &41.7\errmath{0.2} &66.2\\ \midrule
\multirow{2}{*}{MIRO2+KL}  & ERM & SMD&  ImageNet1K     &88.6\errmath{0.1} &71.1\errmath{0.1} &\textbf{44.5}\errmath{0.0} &68.1\\
          & MIRO & SMD & ImageNet1K  &\textbf{89.4}\errmath{0.0} &\textbf{71.6}\errmath{0.1} &44.3\errmath{0.0} &\textbf{68.4}\\
\bottomrule
\end{tabular}

\caption{Performances on DG benchmarks, by adding the KL regularization term to the original MIRO. All averaged accuracies and errors are reported from three best trials.}\label{table: mirokl}
\end{table*}

\begin{table*}[t]\centering

\begin{tabular}{l|l|l|rrrr}\toprule
\multirow{2}{*}{\textbf{Algorithm}}&\multicolumn{1}{c|}{Oracle}&\multicolumn{1}{c|}{Featurizer}&\multicolumn{4}{c}{Benchmark Avg. }  \\
&\multicolumn{1}{c|}{ Pt. Data} & \multicolumn{1}{c|}{ Pt. Data} &PACS & OfficeHome & DomainNet & Avg.\\\midrule
% \multicolumn{15}{l}{\textit{All backbone featurizers are initialized from scratch, including the target task featurizer in Phase 2.} }\\\midrule

%    & 00.0\errmath{0.0} & 00.0\errmath{0.0}& 00.0\errmath{0.0}& 00.0\errmath{0.0}& 00.0\errmath{0.0}} &+0.0 \\ 
MIRO  &ImageNet1K &ImageNet1K                 &87.7\errmath{0.1} &68.9\errmath{0.1} &42.8\errmath{0.1} &66.5\\
\midrule   

MIRO2           &Places365  &ImageNet1K    & 87.4\errmath{0.1} & 66.5\errmath{0.3}& 43.8\errmath{0.0} &65.9\\ 
(Ours)          &SMD        &ImageNet1K    & 88.0\errmath{0.1} & 70.2\errmath{0.2}& 44.3\errmath{0.0}&67.5 \\  \midrule
MIRO2+KL        &Places365  &ImageNet1K   & 87.5\errmath{0.0} & 66.5\errmath{0.2}& 43.9\errmath{0.1}&66.0 \\ 
(Ours)          &SMD        &ImageNet1K    &\textbf{88.6}\errmath{0.1} &\textbf{71.1}\errmath{0.1} &\textbf{44.5}\errmath{0.1} &\textbf{68.1} \\ 

\bottomrule

\end{tabular}
\caption{Performances on DG benchmarks featuring Places365 as oracle pre-training data. All oracle pre-trainings use the ERM method as the Phase 2 Places365-infused oracle is trained from scratch in Phase 1. All averaged accuracies and errors are reported from three best trials.} \label{table: places}

\end{table*}

Table \ref{table: mirokl} summarizes the impact of adding the KL regularization term to the original 1-phase MIRO. We find out the MIRO+KL setup that adds the KL regularization term alone actually brings down performances especially on PACS and DomainNet, and its average of the three benchmarks remains close to the original MIRO baseline. Therefore, we have shown the necessity that the additive KL regularization term be used together with oracle pre-training such as the MIRO2+KL method.

\subsection{The Effects of Oracle Pre-training with Scene Based Dataset}

We examine the effect of oracle pre-training data brought by large scene-based image classification dataset. We choose Places365-Standard (Places365 for short) created by \citep{places}, which features approximately 2 millions images categorized in 365 types of real-life scenes, roughly twice the size of ImageNet1K and 25 times of SMD. We obtain the Places365 pre-trained oracle by training a ResNet50 backbone featurizer from scratch using ERM. We report the performances on PACS, OfficeHome, and DomainNet benchmarks in comparison with the baseline ImageNet1K MIRO, and the MIRO2 and MIRO2+KL variants that similarly use ERM-based oracle pre-training from scratch.

As is shown in Table \ref{table: places}, we find under the same pre-training methods, using the vast scene dataset Places365 for oracle pre-training results in an overall inferior performance on all three DG benchmarks, even failing to surpass the baseline MIRO. We have thus further demonstrated the superiority of using our SMD as oracle pre-training data on DG tasks.
